# Supplementary material for: Quantum transduction with adaptive control
Source: arXiv:1706.06075 source file (2017-06-20)
Supplement: Supplementary file 1 [file supplement-06-16-17.pdf]

# Supplementary information for "Quantum Transducer with Adaptive Control"

Mengzhen Zhang,[1, 2] Changling Zou,[1, 2, 3] and Liang Jiang[1, 2]

[1] *Departments of Applied Physics and Physics, Yale University, New Haven, CT 06520, USA*

[2] *Yale Quantum Institute, Yale University, New Haven, CT 06520, USA*

[3] *Key Laboratory of Quantum Information, University of Science and Technology of China, CAS, Hefei, Anhui 230026, China*

We provide detailed derivation for the key results. In Sec. S.I, we define the notations. In Sec. S.II, we derive the explicit Gaussian channel representation of the protocol of direct quantum transduction (DQT). In Sec. S.III, we describe the protocol of adaptive quantum transduction (AQT), and then provide the Gaussian channel representation of the AQT protocol with imperfections. In Sec. S.IV, we compare the performances of the minimum realizations of the AQT and DQT protocols, for both beam-splitter type and parametric squeezer type two-mode converters.[S1]

## S.I. NOTATIONS

Given $N$ bosonic modes, there are $N$ pairs of quadrature field operators $\{\hat{q}_k, \hat{p}_k\}_{k=1}^{N}$, formally arranged in the vector

$$\hat{\mathbf{x}} = (\hat{q}_1, \hat{q}_2, \ldots \hat{q}_N; \hat{p}_1, \hat{p}_2, \ldots \hat{p}_N)^T, \tag{S1}$$

where $\hat{q}_k = \hat{c}_k + \hat{c}_k^\dagger$ (Q-quadrature), $\hat{p}_k = -i(\hat{c}_k - \hat{c}_k^\dagger)$ (P-quadrature), $\hat{c}_k$ and $\hat{c}_k^\dagger$ are annihilation and creation operators associated with the $k$-th mode. The canonical commutation relation is

$$[\hat{\mathbf{x}}_j, \hat{\mathbf{x}}_k] = 2i\mathbf{J}_{jk}, \tag{S2}$$

with $\mathbf{J} = \begin{pmatrix} \mathbf{0} & \mathbf{I}_N \\ -\mathbf{I}_N & \mathbf{0} \end{pmatrix}$ and $N \times N$ identity matrix $\mathbf{I}_N$.

A *general Gaussian unitary* $\mathcal{U}_{\mathbf{S},\mathbf{d}}$ is simply described by a map

$$\mathcal{U}_{\mathbf{S},\mathbf{d}}(\hat{\mathbf{x}}) = \mathbf{S}\hat{\mathbf{x}} + \mathbf{d}, \tag{S3}$$

where $\mathbf{d} \in \mathbb{R}^{2N}$ is the displacement vector and $\mathbf{S} \in \mathrm{Sp}(2N, \mathbb{R})$ is a symplectic (scattering) matrix satisfying $\mathbf{SJS^T} = \mathbf{J}$ [S2]. The general Gaussian unitary preserves the canonical commutation relations. Any general Gaussian unitary can be decomposed as a Gaussian unitary (with zero displacement) followed by a displacement operation

$$\mathcal{U}_{\mathbf{S},\mathbf{d}} = \mathcal{U}_{\mathbf{I},\mathbf{d}} \circ \mathcal{U}_{\mathbf{S},\mathbf{0}}. \tag{S4}$$

Since the displacement operation can be easily implemented or compensated experimentally, we will focus on the *Gaussian unitary* (with zero displacement)

$$\mathcal{U}_{\mathbf{S}} := \mathcal{U}_{\mathbf{S},\mathbf{0}}, \tag{S5}$$

which is associated with the symplectic map

$$\mathcal{U}_{\mathbf{S}}(\hat{\mathbf{x}}) = \mathbf{S}\hat{\mathbf{x}}. \tag{S6}$$

Given a symplectic matrix $\mathbf{S}$, there exists a unitary operator $\hat{U}_{\mathbf{S}}$, which is the product of unitary operators $\hat{U}_{\mathbf{S}_i} = \exp\left[-i\hat{\mathbf{x}}^T\mathbf{A}_i\hat{\mathbf{x}}\right]$ with real symmetric matrices $\mathbf{A}_i$s, such that

$$\mathcal{U}_{\mathbf{S}}\left(\hat{O}\right) := \hat{U}_{\mathbf{S}}\hat{O}\hat{U}_{\mathbf{S}}^\dagger \tag{S7}$$

for any operator $\hat{O}$. The symplectic space $E$ associated with the $N$-mode Hilbert space $\mathcal{H}$ is a vector space equipped with a skew inner product $\sigma$. For any two vectors $\mathbf{u}, \mathbf{v} \in E$, the skew inner product is

$$\sigma(\mathbf{u}, \mathbf{v}) = \mathbf{u}^T\mathbf{J}\mathbf{v},$$

which has the following property

$$\sigma(\mathbf{u}, \mathbf{v}) = \sigma(\mathbf{Su}, \mathbf{Sv}) = -\sigma(\mathbf{v}, \mathbf{u}).$$

For the tensor product space $\mathcal{H} = \mathcal{H}_1 \otimes \mathcal{H}_2$, the corresponding symplectic space is $E = E_1 \oplus E_2$, where "$\oplus$" is the symplectic direct sum, defined by

$$\sigma(\mathbf{u}, \mathbf{v}) = \sigma_1(\mathbf{u}_1, \mathbf{v}_1) + \sigma_2(\mathbf{u}_2, \mathbf{v}_2)$$

with $\mathbf{u}, \mathbf{v} \in E$, $\mathbf{u}_1, \mathbf{u}_2, \mathbf{v}_1, \mathbf{v}_2$ the projection of $\mathbf{u}, \mathbf{v}$ on to each subspaces $E_1$ and $E_2$. The largest subspace $l$ of $E$ satisfying $\sigma(\mathbf{u}, \mathbf{u}) = 0$, $\mathbf{u} \in l$, is called Lagrangian plane of $E$, so is its complement $l'$ in $E$, that is $E = l \oplus l'$, $l \cap l' = \{\mathbf{0}\}$.

For a mode converter with bilinear coupling, the outgoing modes are related to the incoming modes via a symplectic (scattering) matrix $\mathbf{S}$ associated with a Gaussian unitary. The incoming modes have $m$ input ports and $n$ ancilla ports, while the outgoing modes have $m$ output ports and $n$ idler ports. In the main text, we use the *expanded notation* to explicitly label the quadratures of the modes— $a\,(a')$ to represent the Q(P)-quadratures of input ports, and similarly $z\,(z')$ for the ancilla ports, $b\,(b')$ for the output ports, and $h\,(h')$ for the idler ports. To simplify the notation, we may also introduce the *compact notation,*

$$in = a \oplus a',\ out = b \oplus b',\ anc = z \oplus z',\ idl = h \oplus h'.$$

Mathematically, the compact notation represents finite-dimension real symplectic spaces, while the expanded spaces represent their corresponding Lagrangian planes

| | Range | Domain |
|---|---|---|
| $\mathbf{S}$ | $\underbrace{h \oplus h'}_{idl} \oplus \underbrace{b \oplus b'}_{out} (\oplus env)$ [a] | $\underbrace{a \oplus a'}_{in} \oplus \underbrace{z \oplus z'}_{anc} (\oplus env)$ |
| $\mathbf{A}$ | $idl \oplus out$ | $in \oplus anc$ |
| $\tilde{\mathbf{S}}$ | $out$ | $in$ |
| $\mathbf{R}$ | $\underbrace{a \oplus a'}_{in'}$ [b] | $out$ |
| $\mathbf{H}$ | $idl \oplus env$ | $idl \oplus env$ |
| $\mathbf{F}(\mathbf{F}^\star)$ | $out$ | $h$ |
| $\mathbf{B}(\mathbf{B}^\star)$ | $in$ | $anc(z)$ |
| $\mathbf{V}_{anc(env)}$ | $anc(env)$ | $anc(env)$ |
| $\mathbf{V}_{in(out)}$ | $in(in')$ | $in(in')$ |
| $\mathbf{V}_{z(z')}$ | $z(z')$ | $z(z')$ |
| $\mathbf{X}_{\mathrm{DQT}}$ | $in'$ | $in$ |
| $\mathbf{Y}_{\mathrm{DQT}}$ | $in'$ | $in'$ |
| $\mathbf{X}_{\mathrm{AQT}}$ | $in'$ | $in$ |
| $\mathbf{Y}_{\mathrm{AQT}}$ | $in'$ | $in'$ |
| $\mathbf{X}_c$ | $in'$ | $out$ |
| $\mathbf{Y}_c$ | $in'$ | $in'$ |

[a] If not explicitly pointed out, *env* will not be included, and the matrix representation will always be organized in this order.
[b] The range of $\mathbf{R}$ is physically different from associated with *in*. In the context, actually $in' = out$. We use this notation to emphasize the signal restoration nature of this operation.

Table I. **Table of domains and ranges of each matrix**

[S3]. Sometimes it is convenient to use the compact notation, while expanded notation is also useful to characterize squeezing and homodyne measurement. Therefore, we will use both compact and expanded notations in our derivation below. In Table I , we list the matrices associated with the linear maps $\mathbf{M} = \mathbf{M}_{b,a}$ from domain $a$ to range $b$.

## S.II. DIRECT QUANTUM TRANSDUCTION

As defined in previous investigations, the matching condition (MC) requires the symplectic matrix fulfills the following conditions: $\mathbf{S}_{out,in} = \mathbf{I}$. Hence, the DQT protocol is imply the identity operation, with the output state equal to the unknown input state

$$\hat{\rho}_{out} = \mathrm{tr}_{idl}(\mathcal{U}_{\mathbf{S}}\left[\hat{\rho}_{in} \otimes \hat{\rho}_{anc}\right]) = \hat{\rho}_{in}, \tag{S8}$$

which corresponds to perfect quantum state transfer [S4, S5]. More generally, we may extend the MC to be $\mathbf{S}_{out,in} = \tilde{\mathbf{S}}$ with some symplectic matrix $\tilde{\mathbf{S}}$, and the DQT protocol is the Gaussian unitary associated with $\tilde{\mathbf{S}}$, with the output state equivalent to the unknown input state up to a unitary transformation $\mathcal{U}_{\tilde{\mathbf{S}}}$.

When the (generalized) MC is not satisfied, we cannot find a unitary operation to faithfully restore the unknown input state. However, if the ancilla modes are initialized in the vacuum state (or other Gaussian states), the DQT protocol can be characterized by a Gaussian channel, which preserves the Gaussian character of a quantum state — transforming Gaussian states into Gaussian states [S2, S6]. Gaussian channel is a larger set of quantum processes, which includes Gaussian unitary as a special case.

A Gaussian state can be fully determined by its first moment (FM) $\bar{\mathbf{x}} = \langle\hat{\mathbf{x}}\rangle$ and covariance matrix (CM) $\mathrm{V}_{ij} = \frac{1}{2}\langle\{\hat{x}_i - \bar{x}_i, \hat{x}_j - \bar{x}_j\}\rangle$, with $\langle\cdot\rangle$ denoting the expectation value and $\{\cdot,\cdot\}$ the anti-commutator. For example, the input Gaussian state has FM $\bar{\mathbf{x}}_{in}$ and CM $\mathbf{V}_{in}$. For the DQT protocol with Gaussian input state and vacuum ancilla, the output state is also Gaussian with the following FM and CM

$$\bar{\mathbf{x}}_{out} = \mathbf{X}_{\mathrm{DQT}}\bar{\mathbf{x}}_{in}, \tag{S9}$$

$$\mathbf{V}_{out} = \mathbf{X}_{\mathrm{DQT}}\mathbf{V}_{in}\mathbf{X}_{\mathrm{DQT}}^T + \mathbf{Y}_{\mathrm{DQT}}, \tag{S10}$$

where the following two matrices

$$\mathbf{X}_{\mathrm{DQT}} = \mathbf{S}_{out,in}, \tag{S11}$$

$$\mathbf{Y}_{\mathrm{DQT}} = \mathbf{S}_{out,anc}\mathbf{S}_{out,anc}^T, \tag{S12}$$

fully characterize the Gaussian channel of DQT [S2, S6].

Later in Sec. S.IV, we will concatenate this DQT channel with a restoration Gaussian channel represented by $\mathbf{X}_{\mathrm{C}}$ and $\mathbf{Y}_{\mathrm{C}}$, to get a new Gaussian channel

$$\mathbf{X}'_{\mathrm{DQT}} = \mathbf{X}_{\mathrm{C}}\mathbf{X}_{\mathrm{DQT}} = \mathbf{I}, \tag{S13}$$

$$\mathbf{Y}'_{\mathrm{DQT}} = \mathbf{X}_{\mathrm{C}}\mathbf{Y}_{\mathrm{DQT}}\mathbf{X}_{\mathrm{C}}^T + \mathbf{Y}_{\mathrm{C}}, \tag{S14}$$

with the compensation channel chosen to minimize $\det \mathbf{Y}'_{\mathrm{DQT}}$. The schematics of DQT channels are shown in Figure S1

## S.III. ADAPTIVE QUANTUM TRANSDUCTION

### A. Perfect AQT

For perfect AQT with infinite squeezing and perfect homodyne detection, we can (1) prepare the ancilla in $|\mathbf{0}\rangle_{\mathbf{x}_z}$, which is an infinitely squeezed state satisfying $\mathbf{x}_z|\mathbf{0}\rangle_{\mathbf{x}_z} = \mathbf{0}|\mathbf{0}\rangle_{\mathbf{x}_z}$, (2) perform perfect homodyne measurement by projecting the idler mode to $|\eta\rangle_{\mathbf{x}_h}$, which is also an infinitely squeezed state satisfying $\mathbf{x}_h|\eta\rangle_{\mathbf{x}_h} = \eta|\eta\rangle_{\mathbf{x}_h}$ with measurement outcome $\eta$, and (3) displace the output modes by $\mathbf{F}_\star\eta$, which is a linear transformation of the measurement outcome $\eta$ with feedforward matrix

$$\mathbf{F}_\star := -\mathbf{S}_{out,z'}\left(\mathbf{S}_{h,z'}\right)^{-1}. \tag{S15}$$

After integrating all possible measurement outcomes, we have the output state:

$$\hat{\rho}_{out} = \int d\eta \mathcal{D}_{\mathbf{F}_\star\eta}\left[\mathrm{tr}_{idl}\left[\mathcal{U}_{\mathbf{S}}\left(\hat{\rho}_{in} \otimes \hat{\rho}_{anc}\right)\hat{\Pi}_\eta\right]\right], \tag{S16}$$

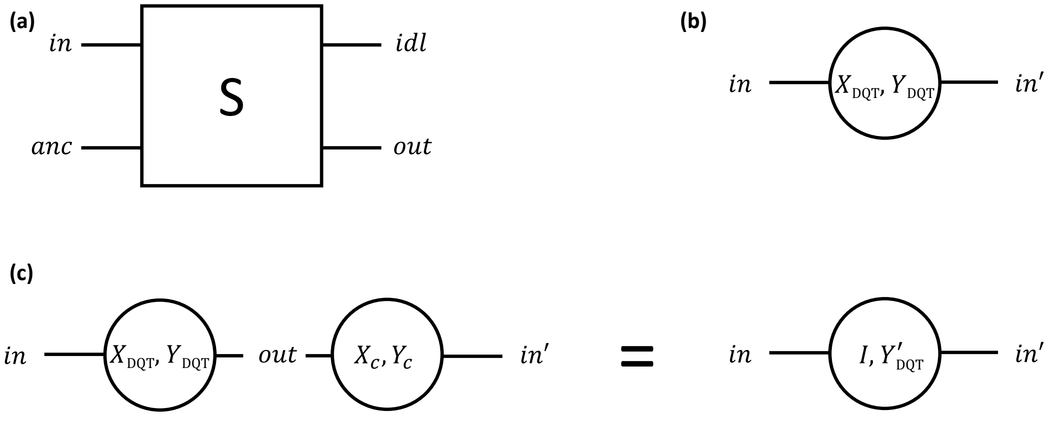


Figure S1. Schematics of DQT. (a) Schematic of the DQT protocol where each horizontal line represents a symplectic space (corresponding to a (multi-mode) Hilbert space) and the square represents a Gaussian unitary. (b) Gaussian channel representation of the DQT protocol. (c) The modified DQT channel as the concatenation of DQT channel with a compensation channel.

where $\hat{\rho}_{anc} = |\mathbf{0}\rangle_{\mathbf{x}_z}\langle\mathbf{0}|$, $\hat{\Pi}_\eta = |\eta\rangle_{\mathbf{x}_h}\langle\eta|$, $\mathcal{U}_\mathbf{S}$ represents the Gaussian unitary of the mode converter, and $\mathcal{D}_{\mathbf{F}_\star\eta}$ represents the adaptive displacement depending on the measurement outcome.

It is convenient to use the Wigner representation to demonstrate the validity of the adaptive protocol. For various Gaussian operations, the Wigner function $W_{\hat{O}}(\mathbf{u})$ of a Hermitian operator $\hat{O}$ has the following properties [S3]:

1. Displacement: $W_{\mathcal{D}_\gamma(\hat{O})}(\mathbf{u}) = W_{\hat{O}}(\mathbf{u}-\gamma)$, with $\mathcal{D}_\gamma\left(\hat{O}\right) = e^{i\mathbf{x}^T\mathbf{J}\gamma}\hat{O}e^{-i\mathbf{x}^T\mathbf{J}\gamma}$ for arbitrary operator $\hat{O}$.

2. Trace and partial trace: $W_{\mathrm{tr}_\alpha(\hat{O}_1\hat{O}_2)}(\mathbf{u}) = \int W_{\hat{O}_1}(\mathbf{u})W_{\hat{O}_2}(\mathbf{u})d\mathbf{u}_\alpha$, with $\alpha$ for the degrees of freedom being traced out.

3. Gaussian unitary: $W_{\mathcal{U}_\mathbf{S}(\hat{O})}(\mathbf{u}) = W_{\hat{O}}(\mathbf{S}^{-1}\mathbf{u})$, with symplectic matrix $\mathbf{S}$ associated with the Gaussian unitary.

4. Tensor product: $W_{\hat{\rho}_1\otimes\hat{\rho}_2}(\mathbf{u}_1 \oplus \mathbf{u}_2) = W_{\hat{\rho}_1}(\mathbf{u}_1)W_{\hat{\rho}_2}(\mathbf{u}_2)$;

5. Ideal squeezed input and homodyne measurement: $W_{\hat{\rho}_{anc}}(\mathbf{u}) = \mathrm{const}\cdot\delta(\mathbf{u})$, $W_{\hat{\Pi}_\eta}(\mathbf{u}) = \mathrm{const}\cdot\delta(\mathbf{u}-\eta)$.

Using the above properties, we obtain

$$W_{\mathrm{tr}_{idl}\left[\mathcal{U}_\mathbf{S}(\hat{\rho}_{in}\otimes\hat{\rho}_{anc})\hat{\Pi}_\eta\right]}(\mathbf{u}) \propto W_{\hat{\rho}_{in}}\left(\tilde{\mathbf{S}}^{-1}\mathbf{u}_{out} + \mathbf{F}_\star\eta\right), \tag{S17}$$

where

$$\tilde{\mathbf{S}} := \mathbf{S}_{out,in} + \mathbf{F}_\star\mathbf{S}_{h,in}. \tag{S18}$$

After performing the adaptive displacement operation $\mathcal{D}_{\mathbf{F}_*\eta}$, we have

$$W_{\hat{\rho}_{out}}(\mathbf{u}_{out}) = W_{\hat{\rho}_{in}}\left(\tilde{\mathbf{S}}^{-1}\mathbf{u}_{out}\right). \tag{S19}$$

For symplectic $\tilde{S}$, we have $W_{\hat{\rho}_{out}}(\mathbf{u}_{out}) = W_{\mathcal{U}_{\tilde{\mathbf{S}}}(\hat{\rho}_{in})}(\mathbf{u}_{out})$ using property 3, which implies that $\hat{\rho}_{out} = \mathcal{U}_{\tilde{\mathbf{S}}}(\hat{\rho}_{in})$ is equalvant to $\hat{\rho}_{in}$ up to a Gaussian unitary. As shown in the main text, $\tilde{\mathbf{S}}$ is indeed a symplectic matrix. Using Theorem. 1. which will be proved later, we may conclude that there is a Gaussian unitary to restore the input state from the output, $\mathcal{U}_\mathbf{R}(\hat{\rho}_{out}) = \hat{\rho}_{in}$ with symplectic matrix $\mathbf{R} = \tilde{\mathbf{S}}^{-1}$. The schematic of the perfect AQT is shown in Figure S2.

Now we prove the theorem:

**Theorem 1.** Given a symplectic matrix $\mathbf{S}$: $in \oplus anc \to out \oplus idl$, where $\dim(in) = \dim(out)$, $anc = z \oplus z'$, $idl = h \oplus h'$, and $\bar{\mathbf{S}} := \mathbf{S}^{-1}$, with invertible block matricies $\mathbf{S}_{h,z'}$ . Then

$$\tilde{S}_{out,in} := \mathbf{S}_{out,in} - \mathbf{S}_{out,z'}(\mathbf{S}_{h,z'})^{-1}\mathbf{S}_{h,in} \tag{S20}$$

$$\tilde{\bar{S}}_{in,out} := \bar{\mathbf{S}}_{in,out} - \bar{\mathbf{S}}_{in,h'}(\bar{\mathbf{S}}_{z,h'})^{-1}\bar{\mathbf{S}}_{z,out} \tag{S21}$$

are symplectic matrices, which are inverses of each other

$$\tilde{\bar{\mathbf{S}}}\tilde{\mathbf{S}} = \mathbf{I}. \tag{S22}$$

**Proof.** We prove the theorem in the following three steps: (1) show $\tilde{S}_{out,in}$ is symplectic, (2) show $\tilde{\bar{S}}_{in,out}$ is symplectic, and (3) show they are inverses of each other.

(1) For $\mathbf{u} \in in \oplus anc$, $\mathbf{v} \in out \oplus idl$, the map $\mathbf{S}$ can be explicitly expressed as

$$\begin{pmatrix} \mathbf{v}_{out} \\ \mathbf{v}_h \\ \mathbf{v}_{h'} \end{pmatrix} = \begin{pmatrix} \mathbf{S}_{out,in} & \mathbf{S}_{out,z} & \mathbf{S}_{out,z'} \\ \mathbf{S}_{h,in} & \mathbf{S}_{h,z} & \mathbf{S}_{h,z'} \\ \mathbf{S}_{h',in} & \mathbf{S}_{h',z} & \mathbf{S}_{h',z'} \end{pmatrix} \begin{pmatrix} \mathbf{u}_{in} \\ \mathbf{u}_z \\ \mathbf{u}_{z'} \end{pmatrix}. \tag{S23}$$

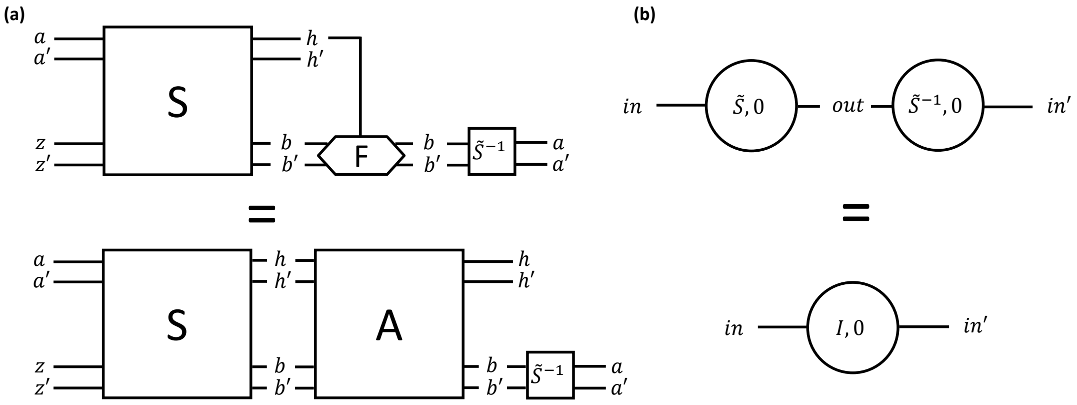


Figure S2. Schematic of perfect AQT. (a) Two Equivalent representations of the perfect AQT protocol where each line represents a Lagrangian plane, each square represents a Gaussian unitary defined in the text. (b) Schematic of the Gaussian channel representation of the perfect AQT.

Given arbitrary $\mathbf{w} \in in$, we assign $\mathbf{u}_{in} = \mathbf{w}$, $\mathbf{u}_z = \mathbf{0}$, $\mathbf{u}_{z'} = \mathbf{F}'\mathbf{w}$, and $\mathbf{F}' = -(\mathbf{S}_{h,z'})^{-1}\mathbf{S}_{h,in}$. Plug into Eq.(S23), we have

$$\begin{pmatrix} \mathbf{v}_{out} \\ \mathbf{v}_h \\ \mathbf{v}_{h'} \end{pmatrix} = \begin{pmatrix} \tilde{\mathbf{S}}\mathbf{w} \\ \mathbf{0} \\ \mathbf{S}''\mathbf{w} \end{pmatrix}, \tag{S24}$$

with $\tilde{\mathbf{S}}_{out,in} = \mathbf{S}_{out,in} - \mathbf{S}_{out,z'}(\mathbf{S}_{h,z'})^{-1}\mathbf{S}_{h,in}$ and

$$\mathbf{S}'' = \left(\mathbf{S}_{h',in} - \mathbf{S}_{h',z'}(\mathbf{S}_{h,z'})^{-1}\mathbf{S}_{h,in}\right). \tag{S25}$$

Similarly, for arbitrary $\mathbf{w}' \in in$, we assign $\mathbf{u}'_{in} = \mathbf{w}'$, $\mathbf{u}'_z = \mathbf{0}$, $\mathbf{u}'_{z'} = \mathbf{F}'\mathbf{w}'$, and we have

$$\begin{pmatrix} \mathbf{v}'_{out} \\ \mathbf{v}'_h \\ \mathbf{v}'_{h'} \end{pmatrix} = \begin{pmatrix} \tilde{\mathbf{S}}\mathbf{w}' \\ \mathbf{0} \\ \mathbf{S}''\mathbf{w}' \end{pmatrix}. \tag{S26}$$

We define the skew inner products $\sigma_{in\oplus anc}(\mathbf{u},\mathbf{u}') := \mathbf{u}^T\mathbf{J}\mathbf{u}$ and $\sigma_{out\oplus idl}(\mathbf{v},\mathbf{v}') := \mathbf{v}^T\mathbf{J}\mathbf{v}$, which are identical as they are invariant under symplectic transformation $\mathbf{u} \rightarrow \mathbf{v} = \mathbf{S}\mathbf{u}$:

$$\begin{aligned} \sigma_{in\oplus anc}(\mathbf{u},\mathbf{u}') &= \mathbf{u}^T\mathbf{J}\mathbf{u} = \mathbf{u}^T\mathbf{S}^T\mathbf{J}\mathbf{S}\mathbf{u} = \mathbf{v}^T\mathbf{J}\mathbf{v} \\ &= \sigma_{out\oplus idl}(\mathbf{v},\mathbf{v}'). \end{aligned} \tag{S27}$$

Meanwhile, we may also simplify the skew inner products:

$$\begin{aligned} &\sigma_{in\oplus anc}(\mathbf{u},\mathbf{u}') \\ &= \begin{pmatrix} \mathbf{w} \\ \mathbf{0} \\ \mathbf{F}'\mathbf{w} \end{pmatrix}^T \begin{pmatrix} \mathbf{J}_{in,in} & & \\ & \mathbf{0} & \mathbf{J}_{z,z'} \\ & \mathbf{J}_{z',z} & \mathbf{0} \end{pmatrix} \begin{pmatrix} \mathbf{w}' \\ \mathbf{0} \\ \mathbf{F}'\mathbf{w}' \end{pmatrix} \qquad \text{(S28)} \\ &= \mathbf{w}\mathbf{J}_{in,in}\mathbf{w}' \\ &= \sigma_{in}(\mathbf{w},\mathbf{w}'), \qquad \text{(S29)} \end{aligned}$$

and

$$\begin{aligned} &\sigma_{out\oplus idl}(\mathbf{v},\mathbf{v}') \\ &= \begin{pmatrix} \tilde{\mathbf{S}}\mathbf{w} \\ \mathbf{0} \\ \mathbf{S}''\mathbf{w} \end{pmatrix}^T \begin{pmatrix} \mathbf{J}_{out,out} & & \\ & \mathbf{0} & \mathbf{J}_{h,h'} \\ & \mathbf{J}_{h',h} & \mathbf{0} \end{pmatrix} \begin{pmatrix} \tilde{\mathbf{S}}\mathbf{w}' \\ \mathbf{0} \\ \mathbf{S}''\mathbf{w}' \end{pmatrix} \qquad \text{(S30)} \\ &= \mathbf{w}\tilde{\mathbf{S}}^T\mathbf{J}_{out,out}\tilde{\mathbf{S}}\mathbf{w}' \\ &= \sigma_{out}\left(\tilde{\mathbf{S}}\mathbf{w}, \tilde{\mathbf{S}}\mathbf{w}'\right). \qquad \text{(S31)} \end{aligned}$$

Therefore, we have

$$\sigma_{in}(\mathbf{w},\mathbf{w}') = \sigma_{out}\left(\tilde{\mathbf{S}}\mathbf{w}, \tilde{\mathbf{S}}\mathbf{w}'\right) \tag{S32}$$

for arbitrary $\mathbf{w}$,$\mathbf{w}' \in in$, which implies $\tilde{\mathbf{S}}^T\mathbf{J}_{out,out}\tilde{\mathbf{S}} = \mathbf{J}_{out,out}$ — that is, $\tilde{\mathbf{S}}$ is symplectic.

(2) Applying $\bar{\mathbf{S}}$ =$\mathbf{S}^{-1}$ to both sides of Eq.(??), we have

$$\begin{pmatrix} \mathbf{u}_{in} \\ \mathbf{u}_z \\ \mathbf{u}_{z'} \end{pmatrix} = \begin{pmatrix} \bar{\mathbf{S}}_{in,out} & \bar{\mathbf{S}}_{in,h} & \bar{\mathbf{S}}_{in,h'} \\ \bar{\mathbf{S}}_{z,out} & \bar{\mathbf{S}}_{z,h} & \bar{\mathbf{S}}_{z,h'} \\ \bar{\mathbf{S}}_{z',out} & \bar{\mathbf{S}}_{z',h} & \bar{\mathbf{S}}_{z',h'} \end{pmatrix} \begin{pmatrix} \mathbf{v}_{out} \\ \mathbf{v}_h \\ \mathbf{v}_{h'} \end{pmatrix}. \tag{S33}$$

Similar to part (1), we assign $\mathbf{v}_{out} = \mathbf{z}$, $\mathbf{v}_h = \mathbf{0}$, $\mathbf{v}_{h'} = \bar{\mathbf{F}}'\mathbf{z}$, and $\bar{\mathbf{F}}' = -(\bar{\mathbf{S}}_{z,h'})^{-1}\bar{\mathbf{S}}_{z,out}$. For arbitrary $\mathbf{z},\mathbf{z}' \in out$, we can show $\sigma_{out}(\mathbf{z},\mathbf{z}') = \sigma_{in}\left(\tilde{\bar{\mathbf{S}}}\mathbf{z}, \tilde{\bar{\mathbf{S}}}\mathbf{z}'\right)$ with

$$\tilde{\bar{\mathbf{S}}} = \bar{\mathbf{S}}_{in,out} - \bar{\mathbf{S}}_{in,h'}(\bar{\mathbf{S}}_{z,h'})^{-1}\bar{\mathbf{S}}_{z,out}. \tag{S34}$$

Therefore, $\tilde{\bar{\mathbf{S}}}$ is a symplectic matrix.

Similar to part (1), here we also require $\bar{\mathbf{S}}_{z,h'}$ is invertible. But there is no need to make this as another assumption since it's guaranteed by the invertibility of $\mathbf{S}_{h,z'}$. This can be shown by directly using the definition, $\mathbf{S}^T\mathbf{J}\mathbf{S} = \mathbf{J}$, which leads to $\bar{\mathbf{S}} = -\mathbf{J}\mathbf{S}^T\mathbf{J}$. So by direct calculation, we get $\bar{\mathbf{S}}_{z,h'} = -\mathbf{J}_{z,z'}(\mathbf{S}_{h,z'})^T\mathbf{J}_{h,h'}$. Thus the invertibility of $\mathbf{S}_{h,z'}$ leads to the invertibility of $\bar{\mathbf{S}}_{z,h'}$.

(3) We assign $\mathbf{u}_{in}=\mathbf{w}$, $\mathbf{u}_{z}=\mathbf{0}$, $\mathbf{u}_{z'}=\mathbf{F}'\mathbf{w}$, for arbitrary $\mathbf{w}\in in$. Following Eq.(??), $\mathbf{v}_{out}=\tilde{\mathbf{S}}\mathbf{w}$, $\mathbf{v}_{h}=\mathbf{0}$, $\mathbf{v}_{h'}=\mathbf{S}''\mathbf{w}$. Applying Eq.(S33), we have

$$\mathbf{u}_{in}=\left(\bar{\mathbf{S}}_{in,out}\tilde{\mathbf{S}}+\bar{\mathbf{S}}_{in,h'}\mathbf{S}''\right)\mathbf{w}=\mathbf{w} \tag{S35}$$

$$\mathbf{u}_{z}=\left(\bar{\mathbf{S}}_{z,out}\tilde{\mathbf{S}}+\bar{\mathbf{S}}_{z,h'}\mathbf{S}''\right)\mathbf{w}=0. \tag{S36}$$

Since the these two equations are satisifed for abitrary $\mathbf{w}$, we have

$$\left(\bar{\mathbf{S}}_{in,out}\tilde{\mathbf{S}}+\bar{\mathbf{S}}_{in,h'}\mathbf{S}''\right)=\mathbf{I} \tag{S37}$$

$$\bar{\mathbf{S}}_{z,out}\tilde{\mathbf{S}}+\bar{\mathbf{S}}_{z,h'}\mathbf{S}''=\mathbf{0}. \tag{S38}$$

For invertible $\bar{\mathbf{S}}_{z,h'}$, we have $\left(\bar{\mathbf{S}}_{in,out}-\bar{\mathbf{S}}_{in,h'}\left(\bar{\mathbf{S}}_{z,h'}\right)^{-1}\bar{\mathbf{S}}_{z,out}\right)\tilde{\mathbf{S}}=\mathbf{I}$, which is $\tilde{\tilde{\mathbf{S}}}\tilde{\mathbf{S}}=\mathbf{I}$. Therefore, $\tilde{\mathbf{S}}$ and $\tilde{\tilde{\mathbf{S}}}$ are inverses of each other.□

### B. Imperfect AQT

First, we develop a general formalism for the AQT with adaptive displacement that linearly depends on the homodyne measurement outcome. In the presence of imperfections, we will optimize the choice of feed-forward matrix $\mathbf{F}$ (not necessarily the same as $\mathbf{F}_*$ for the perfect AQT), which determines the adaptive displacement $\mathbf{F}\eta$ conditioned on measurement outcome $\eta$. We consider the Wigner function of the output state

$$\begin{aligned}
&W_{\hat{\rho}'}(\mathbf{u}_{out})\\
&\propto\int\int\int W_{\hat{\rho}}\begin{pmatrix}\mathbf{u}_{out}-\mathbf{F}\eta\\ \mathbf{u}_{h}\\ \mathbf{u}_{h'}\end{pmatrix}\delta(\mathbf{u}_{h}-\eta)d\mathbf{u}_{h}d\mathbf{u}_{h'}d\eta\\
&=\int\int W_{\hat{\rho}}\begin{pmatrix}\mathbf{u}_{out}-\mathbf{F}\mathbf{u}_{h}\\ \mathbf{u}_{h}\\ \mathbf{u}_{h'}\end{pmatrix}d\mathbf{u}_{h}d\mathbf{u}_{h'}\\
&=\int\int W_{\hat{\rho}}(\begin{pmatrix}\mathbf{u}_{out}-\mathbf{F}\mathbf{u}_{h}\\ \mathbf{u}_{h}\\ \mathbf{E}\mathbf{u}_{out}+\mathbf{G}\mathbf{u}_{h}+\mathbf{u}_{h'}\end{pmatrix})d\mathbf{u}_{h}d\mathbf{u}_{h'}\\
&=\int\int W_{\hat{\rho}}\left(\mathbf{A}^{-1}\begin{pmatrix}\mathbf{u}_{out}\\ \mathbf{u}_{h}\\ \mathbf{u}_{h'}\end{pmatrix}\right)d\mathbf{u}_{h}d\mathbf{u}_{h'}\\
&=\int\int W_{\mathcal{U}_{\mathbf{A}}(\hat{\rho})}\left(\begin{pmatrix}\mathbf{u}_{out}\\ \mathbf{u}_{h}\\ \mathbf{u}_{h'}\end{pmatrix}\right)d\mathbf{u}_{h}d\mathbf{u}_{h'}
\end{aligned} \tag{S39}$$

where $A$ is a symplectic matrix

$$\mathbf{A}=\begin{pmatrix}\mathbf{I}_{out}&\mathbf{F}&\\ &\mathbf{I}_{h}&\\ -\mathbf{E}&\mathbf{G}&\mathbf{I}_{h'}\end{pmatrix} \tag{S40}$$

with $\mathbf{E}=-\mathbf{J}_{h',h}\mathbf{F}^{T}\mathbf{J}_{out,out}$, $\mathbf{G}=\frac{1}{2}\mathbf{J}_{h',h}\mathbf{F}^{T}\mathbf{J}_{out,out}\mathbf{F}$, and $\mathbf{J}_{h',h}$, $\mathbf{J}_{out,out}$, $\mathbf{J}_{h,h'}$ for the subblocks of the fundamental symplectic matrix $\mathbf{J}$. In the second equality, we shifted $\mathbf{u}_{h}'$ by $\mathbf{E}\mathbf{u}_{out}+\mathbf{G}\mathbf{u}_{h}$ without changing the integral. In the third equality, we introduce

$$\mathbf{A}^{-1}=\begin{pmatrix}\mathbf{I}_{out}&-\mathbf{F}&\\ &\mathbf{I}_{h}&\\ \mathbf{E}&\mathbf{G}&\mathbf{I}_{h'}\end{pmatrix},$$

which is the inverse of $A$, as $\mathbf{E}\mathbf{F}+2\mathbf{G}=\mathbf{0}$. Eq.(S39) implies that the channel of AQT with feed-forward matrix $\mathbf{F}$ is the same as the Gaussian unitary associated with $A$ followed by tracing out the idler modes.

Now we consider the two major imperfections: (1) First, the ancilla starts in some Gaussian state with *finite* squeezing, characterized by the CM $\mathbf{V}_{anc}=\begin{pmatrix}\mathbf{V}_{z}&\mathbf{0}\\ \mathbf{0}&\mathbf{V}_{z'}\end{pmatrix}$, with a positive matrix $\mathbf{V}_{z}=e^{-2\xi}\left(2n_{z}+1\right)\mathbf{I}$ for finite squeezing. For simplicity, we introduce the parameter

$$\nu=e^{-2\xi}\left(2n_{z}+1\right)$$

to characterize the imperfection in squeezing. (2) In addition, the imperfect homodyne detector has limited efficiency, characterized by the parameter $\eta\in[0,1]$. We also introduce the parameter

$$\mu=\frac{1-\eta}{\eta}$$

to characterize the measurement imperfection.

The imperfect homodyne detector with efficiency $\eta$ behaves exactly the same as a perfect homodyne detector preceed by a beam splitter (BS) that mixes the input signal with some vacuum noise from the envirnoment port ($env$). The beam splitter with transmittance $\eta$ is a Gaussian unitary $\mathcal{U}_{\mathbf{H}}$ with a symplectic matrix

$$\mathbf{H}=\begin{pmatrix}\sqrt{\eta}&\sqrt{1-\eta}\\ -\sqrt{1-\eta}&\sqrt{\eta}\end{pmatrix}\otimes\mathbf{I}_{2} \tag{S41}$$

characterizing the coupling between the idler and vacuum envinorment. For vacuum environment, $\hat{\rho}_{env}=|vac\rangle\langle vac|$ and $\mathbf{V}_{env}=\begin{pmatrix}1&\mathbf{0}\\ \mathbf{0}&1\end{pmatrix}$. Therefore, the general AQT can be represented as:

$$\hat{\rho}_{out}=\mathcal{G}\left(\hat{\rho}_{in}\right)=\mathrm{tr}_{idl\otimes env}\left(\mathcal{U}_{\mathbf{A}}\circ\mathcal{U}_{\mathbf{H}}\circ\mathcal{U}_{\mathbf{S}}\left(\hat{\rho}_{in}\otimes\hat{\rho}_{anc}\otimes\hat{\rho}_{env}\right)\right), \tag{S42}$$

where the Gaussian unitaries are determined by the responding symplectic matrix (e.g., Eqs.(S40,S41)).

The general AQT is a Gaussian channel $\mathcal{G}$, because its characterization (Eq(S42)) only uses Gaussian unitaries ($\mathcal{U}_{\mathbf{A}}$, $\mathcal{U}_{\mathbf{S}}$ and $\mathcal{U}_{\mathbf{H}}$) and Gaussian ancillary states ($\hat{\rho}_{anc}$ and $\hat{\rho}_{env}$) [S2, S6]. Similar to the DQT Gaussian channel (Eqs.S11S12), we just need two matrices to fully characterize the general AQT

$$\mathbf{X}_{\mathrm{AQT}} = \mathbf{S}_{out,in} + \sqrt{\eta}\mathbf{F}\mathbf{S}_{h,in} \tag{S43}$$

$$\mathbf{Y}_{\mathrm{AQT}} = \nu\mathbf{B}\mathbf{B}^{T} + (1-\eta)\,\mathbf{F}\mathbf{F}^{T}, \tag{S44}$$

with

$$\mathbf{B} := \mathbf{S}_{out,anc} + \sqrt{\eta}\mathbf{F}\mathbf{S}_{h,anc}. \tag{S45}$$

If needed, we may apply a gaussian unitary $\mathcal{U}_{\mathbf{R}}$ associated with a symplectic matrix $\mathbf{R}$ to restore the quantum signal. For the case of perfect AQT with $\mathbf{F} = \mathbf{F}_{*}$, $\mathbf{X}_{\mathrm{AQT}} = \tilde{\mathbf{S}}$ is a symplectic matrix and we simply choose $\mathbf{R} = \tilde{\mathbf{S}}^{-1}$ for restoration. For imperfect AQT, we need to optimize the choice of $\mathbf{F}$ and $\mathbf{R}$ for the best performance. To evaluate the performance of the AQT, we may use the input-output fidelity averaged over uniformly distributed coherent states (i.e., average fidelity over all coherent states) and quantum channel capacity.

### C. Average Fidelity over All Coherent States

To have a non-vanishing average fidelity over all coherent states, we should be able to restore the FM for all coherent states, which implies $\mathbf{R}\mathbf{X}_{\mathrm{AQT}} = \mathbf{I}$. If we assume $\mathbf{R}$ is a symplectic matrix, then $\mathbf{X}_{\mathrm{AQT}}$ should be symplectic, which can be fulfilled by choosing

$$\mathbf{F} = \eta^{-1/2}\mathbf{F}_{\star}, \tag{S46}$$

so that

$$\mathbf{X}_{\mathrm{AQT}} = \tilde{\mathbf{S}}.$$

Moreover, such choice of $\mathbf{F}$ complete eliminantes of noise from anti-squeezed quadratures, and mathematically we have $\mathbf{B} = \begin{pmatrix} \tilde{\mathbf{S}}\mathbf{B}_{\star} \\ \mathbf{0} \end{pmatrix}$ and

$$\begin{aligned} \mathbf{B}_{\star} &= \tilde{\mathbf{S}}^{-1}(\mathbf{S}_{out,z} - \mathbf{S}_{out,z'}\left(\mathbf{S}_{h,z'}\right)^{-1}\mathbf{S}_{h,z}) \\ &= -\bar{\mathbf{S}}_{in,h'}\left(\bar{\mathbf{S}}_{z,h'}\right)^{-1}. \end{aligned} \tag{S47}$$

where $\bar{\mathbf{S}}_{in,h'} = \left(\mathbf{S}^{-1}\right)_{in,h'}$, $\bar{\mathbf{S}}_{z,h'} = \left(\mathbf{S}^{-1}\right)_{z,h'}$, and the second equality in the calculation of $\mathbf{B}_{\star}$ is justified by Proposition 2, which will be shown later. . (The elimination of noise from anti-squeezed quadratures is especailly useful when the squeezing is good.) Hence, there will only be noises from the squeezed quadratures and imperfect homodyne measurement contributing to the CM

$$\mathbf{Y}_{\mathrm{AQT}} = \nu\tilde{\mathbf{S}}\mathbf{B}_{\star}\mathbf{B}_{\star}^{T}\tilde{\mathbf{S}}^{T} + \mu\mathbf{F}_{\star}\mathbf{F}_{\star}^{T}. \tag{S48}$$

with $\mu = \frac{1-\eta}{\eta}$ to characterize the measurement imperfection.

After the restoration with $\mathbf{R} = \tilde{\mathbf{S}}^{-1}$, we have

$$\mathbf{X}'_{\mathrm{AQT}} = \mathbf{R}\mathbf{X}_{\mathrm{AQT}} = \mathbf{I}, \tag{S49}$$

$$\mathbf{Y}'_{\mathrm{AQT}} = \nu\mathbf{B}_{\star}\left(\mathbf{B}_{\star}\right)^{T} + \mu\tilde{\mathbf{S}}^{-1}\mathbf{F}_{\star}\mathbf{F}_{\star}^{T}\left(\tilde{\mathbf{S}}^{-1}\right)^{T}. \tag{S50}$$

Therefore, the combined process of AQT and restoration is a *classical-noise channel* [S2], transforming the quadratures as $\hat{\mathbf{x}} \to \hat{\mathbf{x}} + \xi$, where $\xi$ is Gaussian noise with for the CM of $\mathbf{Y}'_{\mathrm{AQT}}$ (Eq.(S50)), which is the explicit form used in the main text.

For intuitive understanding of the added noise, we may draw a schematic to track the flow of added noise. As illustred in Fig. S3, we may attribute the first term in Eq. (S50) to the noise from the squeezed quadrature, which is transformed under $\mathbf{B}_{\star} = -\bar{\mathbf{S}}_{in,h'}\left(\bar{\mathbf{S}}_{z,h'}\right)^{-1}$. and added to the input port of the perfect AQT. Similarly, we may attribute the second term in Eq. (S50) to the noise from the homodyne measurement, which is transformed under $\mathbf{F}_{\star} = -\mathbf{S}_{out,z'}\left(\mathbf{S}_{h,z'}\right)^{-1}$ (before the restoration $\mathbf{R} = \tilde{\mathbf{S}}^{-1}$) and then added to the output port of the perfect AQT.

The validity of this concise form is shown here:

$$\mathbf{S}'' = \left(\mathbf{S}_{h',in} - \mathbf{S}_{h',z'}(\mathbf{S}_{h,z'})^{-1}\mathbf{S}_{h,in}\right). \tag{S51}$$

**Proposition 2.** Given a symplectic map $\mathbf{S}$: $in \oplus anc \to out \oplus idl$, with $\dim(in) = \dim(out)$, $anc = z \oplus z'$, $idl = h \oplus h'$, and the inverse map $\bar{\mathbf{S}} = \mathbf{S}^{-1}$. For invertible block matricies $\mathbf{S}_{h,z'}$ , the block matrices of $\mathbf{S}$ and $\bar{\mathbf{S}}$ satisfy the following to relations:

$$-\bar{\mathbf{S}}_{in,h'}\left(\bar{\mathbf{S}}_{z,h'}\right)^{-1} = \tilde{\mathbf{S}}^{-1}(\mathbf{S}_{out,z} - \mathbf{S}_{out,z'}\left(\mathbf{S}_{h,z'}\right)^{-1}\mathbf{S}_{h,z}) \tag{S52}$$

and

$$-\mathbf{S}_{out,z'}\left(\mathbf{S}_{h,z'}\right)^{-1} = \tilde{\mathbf{S}}(\bar{\mathbf{S}}_{in,h} - \bar{\mathbf{S}}_{in,h'}\left(\bar{\mathbf{S}}_{z,h'}\right)^{-1}\bar{\mathbf{S}}_{z,h}). \tag{S53}$$

**Proof.** We apply $\bar{\mathbf{S}}$ to Eq.(**??**) to get

$$\mathbf{u}_{z} = \left[\bar{\mathbf{S}}_{z,h'}\mathbf{S}'' + \bar{\mathbf{S}}_{z,out}\tilde{\mathbf{S}}\right]\mathbf{w} = \mathbf{0}, \tag{S54}$$

which implies

$$-\left(\bar{\mathbf{S}}^{T}\right)_{out,z}\left(\left(\bar{\mathbf{S}}^{T}\right)_{h',z}\right)^{-1} = \left(\tilde{\mathbf{S}}^{T}\right)^{-1}\left(\mathbf{S}''\right)^{T}. \tag{S55}$$

Then we can commute transposition operation with the operations of $\bar{\square}$, $\tilde{\square}$, and $\square''$, which can be justified as follows. Since $\bar{\mathbf{S}} = \mathbf{S}^{-1}$, we have

$$\bar{\mathbf{S}}^{T} = \left(\mathbf{S}^{-1}\right)^{T} = \left(\mathbf{S}^{T}\right)^{-1} = \overline{\mathbf{S}^{T}}. \tag{S56}$$

And according to the definitions of Eqs.(S18,**??**), we have

$$\begin{aligned} &\tilde{\mathbf{S}}^{T} \\ &= \left(\mathbf{S}^{T}\right)_{in,out} - \left(\mathbf{S}^{T}\right)_{in,h}\left(\left(\mathbf{S}^{T}\right)_{z',h}\right)^{-1}\left(\mathbf{S}^{T}\right)_{z',out} \\ &= \widetilde{\mathbf{S}^{T}} \end{aligned} \tag{S57}$$

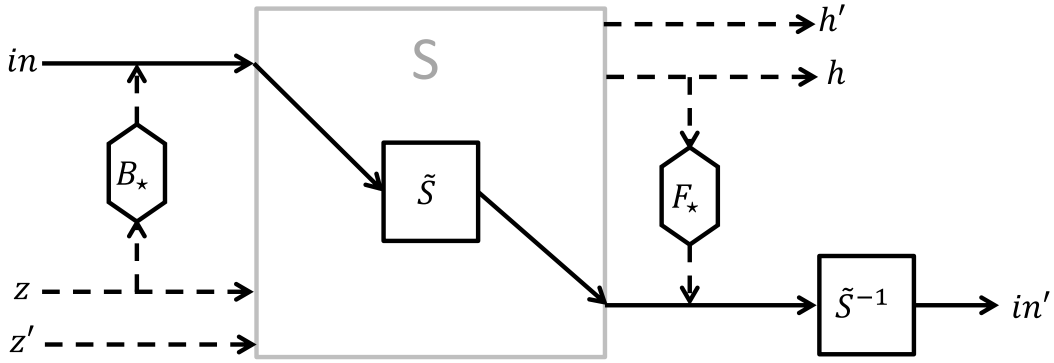


Figure S3. Schematics of noise sources. Each solid arrow represents the signal flow, while each dashed arrow represents the noise flow. The squares represent the Gaussian unitary processes. The hexagons represent forward and backward transmission of noise from ancillary modes to signals.

and

$$\begin{aligned} &(\mathbf{S}'')^{T} \\ &= (\mathbf{S}^T)_{in,h'} - (\mathbf{S}^T)_{in,h}\left((\mathbf{S}^T)_{z',h}\right)^{-1}(\mathbf{S}^T)_{z',h'} \\ &= (\mathbf{S}^T)''. \end{aligned} \tag{S58}$$

Hence, Eq.(S55) can be rewritten as

$$-\left(\overline{\mathbf{S}^T}\right)_{out,z}\left(\left(\overline{\mathbf{S}^T}\right)_{h',z}\right)^{-1} = \left(\widetilde{S^T}\right)^{-1}(\mathbf{S}^T)''. \tag{S59}$$

After replacing $\mathbf{S}^T$ with $\mathbf{S}$, we have

$$\begin{aligned} &-\bar{\mathbf{S}}_{out,z}\left(\bar{\mathbf{S}}_{h',z}\right)^{-1} \\ &= \tilde{\mathbf{S}}^{-1}\mathbf{S}'' \\ &= \tilde{\mathbf{S}}^{-1}\left(\mathbf{S}_{in,h'} - \mathbf{S}_{in,h}(\mathbf{S}_{z',h})^{-1}\mathbf{S}_{z',h'}\right). \end{aligned} \tag{S60}$$

Finally, we relabel the indices (i.e., exchanging $in$ with $out$, $z$ with $h'$, and $z'$ with $h$) and obtain Eq.(S52).

Similarly, we can obtain Eq.(S53) by replacing $\mathbf{S}^T$ with $\bar{\mathbf{S}}$ in Eq.(S59) and exchanging $z$ with $z'$ and $h$ with $h'$.□

## S.IV. PERFORMANCE COMPARISON OF IMPERFECT AQT WITH DQT

The first figure of merit we use to calibrate the performance is the average fidelity of transferring coherent states that are uniformly distributed in the phase space. Using the formula given by Ref. [S7], for a single mode Gaussian channel described by pair of matrices $\mathbf{X}$ and $\mathbf{Y}$, this quantity can be expressed as

$$F = \begin{cases} \frac{2}{\sqrt{\det(2\mathbf{I}+\mathbf{Y})}} & \text{if } \mathbf{X} = \mathbf{I}, \\ 0 & \text{if } \mathbf{X} \neq \mathbf{I}. \end{cases} \tag{S61}$$

However, for the Gaussian channel representation of DQT, $\mathbf{X}_{\text{DQT}}$ is not necessarily an identity matrix. To make a fair comparison, we can concatenate it with another Gaussian channel to compensate the undesired dilatation of the first moment. The optimal compensated channel we get is denoted by $\mathbf{X}'_{\text{DQT}}$ and $\mathbf{Y}'_{\text{DQT}}$, as defined in Eqs.(S13,S14).

The second figure of merit is quantum channel capacity $Q$. For a single mode Gaussian channel with $\det(\mathbf{X}) \neq 1$, the lower bound of the quantum channel capacity is given by Ref. [S8], which can be tight for all degradable and anti-degradable channels; for $\det(\mathbf{X}) = 1$, a lower bound is shown in Ref. [S9] as $Q \geq \frac{1}{2}\log_2\left(1 + 2/\sqrt{\det \mathbf{Y}}\right) - 1$. For the comparison of channel capacity, we will use unoptimized, Gaussian channel ($\mathbf{X}_d$, $\mathbf{Y}_d$) for DQT as defined in Eqs.(S11,S12).

In the following subsections, we use these two figures of merit (average fidelity and quantum channel capacity) to compare the performance of DQT and AQT (with imperfect squeezing and homodyne detection). We consider mode converters with two typical bilinear couplings — (1) beam splitter coupling and (2) two-mode squeezer coupling.

### A. Mode converter with beam splitter coupling

For a mode converter with beam splitter coupling ($\hat{H} = g\left(a_1^\dagger a_2 + h.c.\right)$), we use the input-output theory to calculate the scattering matrix

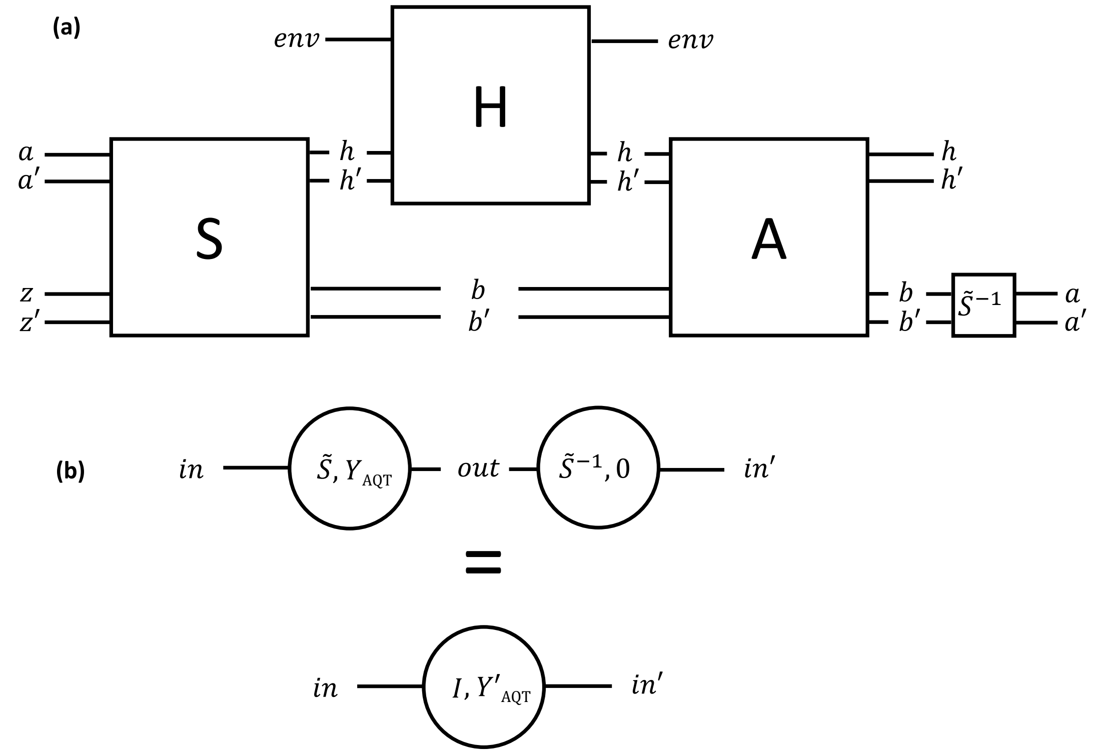


Figure S4. Schematic of imperfect AQT. a. The imperfect AQT protocol with each horizontal line representing the Q-quadratures and P-quadratures, each square representing a Gaussian unitary. b. Schematic of the corresponding Gaussian channel.

$$\mathbf{S}\left(C,\delta\omega\right)=\frac{1}{C+1-4\delta\omega^2}\begin{pmatrix}0 & -2\sqrt{C} & C-1-4\delta\omega^2 & -4\delta\omega\\ 2\sqrt{C} & 0 & -4\delta\omega & C-1-4\delta\omega^2\\ C-1-4\delta\omega^2 & -4\delta\omega & 0 & -2\sqrt{C}\\ -4\delta\omega & C-1-4\delta\omega^2 & 2\sqrt{C} & 0\end{pmatrix}, \tag{S62}$$

where rows are associated with $\{b,b',h,h'\}$ and columns are associated with $\{a,a',z,z'\}$. Here $C=\frac{g^2}{\kappa_1\kappa_2}$, $\delta\omega$ is the detuning from the resonant frequency, $\kappa_{1(2)}$ is the coupling strength of the between input-output channel 1(2) coupled with mode 1(2). Assume resonant coupling with $\delta\omega=0$, we have

$$\mathbf{S}=\begin{pmatrix}0 & -t & r & 0\\ t & 0 & 0 & r\\ r & 0 & 0 & -t\\ 0 & r & t & 0\end{pmatrix}, \tag{S63}$$

where $r=\frac{C-1}{C+1}$, $t=\frac{2\sqrt{C}}{C+1}$, satisfying $r^2+t^2=1$.

For DQT, the Gaussian channel is described by

$$\mathbf{X}_{\mathrm{DQT}}=\begin{pmatrix}\mathbf{S}_{b,a} & \mathbf{S}_{b,a'}\\ \mathbf{S}_{b',a} & \mathbf{S}_{b',a'}\end{pmatrix}=\begin{pmatrix}0 & -t\\ t & 0\end{pmatrix}$$

$$\mathbf{Y}_{\mathrm{DQT}}=\begin{pmatrix}\mathbf{S}_{b,z} & \mathbf{S}_{b,z'}\\ \mathbf{S}_{b',z} & \mathbf{S}_{b',z'}\end{pmatrix}\begin{pmatrix}\mathbf{S}_{b,z} & \mathbf{S}_{b,z'}\\ \mathbf{S}_{b',z} & \mathbf{S}_{b',z'}\end{pmatrix}^T=(1-T)\,\mathbf{I},$$

where $T=t^2\in[0,1]$ is the energy transmittance. For $T>1/2$, DQT is a degradable channel [S10], and the quantum channel capacity is

$$Q_{\mathrm{DQT}}=\max\left\{0,\log_2\frac{T}{1-T}\right\}.$$

The Gaussian channel optimized by additional restoration operation is

$$\mathbf{X}'_{\mathrm{DQT}}=\mathbf{I} \tag{S64}$$

$$\mathbf{Y}'_{\mathrm{DQT}}=2\frac{1-T}{T}\mathbf{I}, \tag{S65}$$

leading to average fidelity

$$F_{\mathrm{DQT}}=T.$$

Then for AQT, by squeezing/measuring the Q-quadrature of the ancilla/idler mode, we get

$$\mathbf{F}_\star=-\begin{pmatrix}\mathbf{S}_{b,z'}\\ \mathbf{S}_{b',z'}\end{pmatrix}\left(\mathbf{S}_{h,z'}\right)^{-1}=-\begin{pmatrix}0\\ r\end{pmatrix}(-t)^{-1}=\begin{pmatrix}0\\ r/t\end{pmatrix}, \tag{S66}$$

$$\tilde{\mathbf{S}} = \begin{pmatrix} \mathbf{S}_{b,a} & \mathbf{S}_{b,a'} \\ \mathbf{S}_{b',a} & \mathbf{S}_{b',a'} \end{pmatrix} + \mathbf{F}_\star \begin{pmatrix} \mathbf{S}_{h,a} & \mathbf{S}_{h,a'} \end{pmatrix} = \begin{pmatrix} 0 & -t \\ t^{-1} & 0 \end{pmatrix}, \tag{S67}$$

and similarly $\mathbf{B}_\star = \begin{pmatrix} 0 \\ r/t \end{pmatrix}$. Notice that $\tilde{\mathbf{S}} = \begin{pmatrix} 0 & -t \\ t^{-1} & 0 \end{pmatrix} = \begin{pmatrix} t & 0 \\ 0 & t^{-1} \end{pmatrix} \begin{pmatrix} 0 & -1 \\ 1 & 0 \end{pmatrix}$ is a product of a single-squeezing operation and $\pi/2$ rotation in the phase space, so to realize AQT, we need to be able to squeeze the corresponding output mode by $\nu_{\tilde{\mathbf{S}}} = 10\log_{10} T\,(\mathrm{dB})$. Actually, all the symplectic transformations can be decomposed into a product of beam splitters, phase shifters and single mode squeezers [S3].

Then, the Gaussian channel including unitary restoration is described by

$$\mathbf{X}'_{\mathrm{AQT}} = \mathbf{I}, \tag{S68}$$

$$\mathbf{Y}'_{\mathrm{AQT}} = (1-T)\begin{pmatrix} \mu & \\ & \nu/T \end{pmatrix}. \tag{S69}$$

The corresponding average fidelity for this channel is

$$F_{\mathrm{AQT}} = \left[\left(1 + \frac{1-T}{2}\mu\right)\left(1 + \frac{1-T}{2T}\nu\right)\right]^{-1/2}, \tag{S70}$$

and the lower bound of its quantum channel capacity is [S9]

$$Q \geq \frac{1}{2}\log_2\left(1 + \frac{2\,(\mu\nu)^{-1/2}}{T^{-1/2} - T^{1/2}}\right) - 1. \tag{S71}$$

### B. Mode converter with two-mode squeezed coupling

For mode converter with two-mode squeezed coupling, we may calculate the scatter matrix. For resonantly coupled modes, the scattering matrix is

$$\mathbf{S} = \begin{pmatrix} 0 & t' & r' & 0 \\ t' & 0 & 0 & r' \\ r' & 0 & 0 & t' \\ 0 & r' & t' & 0 \end{pmatrix}, \tag{S72}$$

where rows are associated with $\{b, b', h, h'\}$ and columns are associated with $\{a, a', z, z'\}$. Here $r' = \frac{C+1}{C-1}$, $t' = \frac{2\sqrt{C}}{1-C}$, satisfying $r'^2 - t'^2 = 1$.

The Gaussian channel obtained by DQT is described by

$$\mathbf{X}_{\mathrm{DQT}} = \begin{pmatrix} 0 & t' \\ t' & 0 \end{pmatrix}, \tag{S73}$$

$$\mathbf{Y}_{\mathrm{DQT}} = (1 + T')\,\mathbf{I}, \tag{S74}$$

where $T' = t'^2 \in [0, \infty)$, which is an anti-degradable channel [S10] and with vanishing channel capacity

$$Q_{\mathrm{DQT}} = 0.$$

To maximize the average fidelity, we apply additional restoration operation and the entire Gaussian channel has

$$\mathbf{X}'_{\mathrm{DQT}} = \mathbf{I}, \tag{S75}$$

$$\mathbf{Y}'_{\mathrm{DQT}} = 2\frac{1+T'}{T'}\mathbf{I}, \tag{S76}$$

leading to an average fidelity

$$F_{\mathrm{DQT}} = \frac{T'}{1+2T'} < 1/2.$$

For AQT, we still squeeze (measure) the Q-quadrature of the ancilla (idler) mode. Then we get

$$\tilde{\mathbf{S}} = \begin{pmatrix} 0 & -t' \\ t'^{-1} & 0 \end{pmatrix}, \tag{S77}$$

$$\mathbf{F}_\star = \begin{pmatrix} 0 \\ -r'/t' \end{pmatrix}, \tag{S78}$$

$$\mathbf{B}_\star = \begin{pmatrix} 0 \\ r'/t' \end{pmatrix}. \tag{S79}$$

Similarly, to implement the restoration, we need squeeze the output quadrature by

$$\nu_{\tilde{\mathbf{S}}} = -10\log_{10} T'\,(\mathrm{dB}).$$

Then the Gaussian channel for the AQT is

$$\mathbf{X}'_{\mathrm{AQT}} = \mathbf{I}, \tag{S80}$$

$$\mathbf{Y}'_{\mathrm{AQT}} = (1+T')\begin{pmatrix} \mu & \\ & \nu/T' \end{pmatrix}, \tag{S81}$$

with average fidelity

$$F = \left[\left(1 + \frac{1+T'}{2}\mu\right)\left(1 + \frac{1+T'}{2T'}\nu\right)\right]^{-1/2}, \tag{S82}$$

and lower bound of quantum channel capacity [S9]

$$Q \geq \frac{1}{2}\log_2\left(1 + \frac{2\,(\mu\nu)^{-1/2}}{T'^{-1/2} + T'^{1/2}}\right) - 1. \tag{S83}$$

[S1] We will not distinguish between the terms linear maps, transformations and matrices throughout this material to reduce the redundancy.

[S2] C. Weedbrook, S. Pirandola, R. García-Patrón, N. J. Cerf, T. C. Ralph, J. H. Shapiro, and S. Lloyd, Rev. Mod. Phys. **84**, 621 (2012).

[S3] M. A. De Gosson, *Symplectic geometry and quantum mechanics*, Vol. 166 (Springer Science & Business Media, 2006).

[S4] A. H. Safavi-Naeini and O. Painter, New J. Phys. **13**, 013017 (2011).

[S5] Y.-D. Wang and A. A. Clerk, Phys. Rev. Lett. **108**, 153603 (2012).

[S6] T. Heinosaari, A. S. Holevo, and M. M. Wolf, Quantum Info. Comput. **10**, 619 (2010).

[S7] C. A. Fuchs and J. v. d. Graaf, IEEE Transactions on Information Theory **45**, 1216 (1999).

[S8] S. Pirandola, R. García-Patrón, S. L. Braunstein, and S. Lloyd, Phys. Rev. Lett. **102**, 050503 (2009).

[S9] J. Harrington and J. Preskill, Phys. Rev. A. **64**, 062301 (2001).

[S10] F. Caruso and V. Giovannetti, Phys. Rev. A 74, 062307 (2006).
